# Supplementary material for: Influence-Driven Data Poisoning in Graph-Based Semi-Supervised Classifiers
Source: arXiv:2012.07381 source file (2022-05-11)
Supplement: Supplementary file 1 [file 8-supplementary.tex]

\section{Supplementary materials}
%\begin{printonly}
Supplementary materials are available in the online version of this paper.
%\end{printonly}

The tables and figures below show our complete empirical results (for RQ2 to RQ4) for three different proportions of labelled inputs (5\%, 15\% and 25\%), whereas the tables and figures presented in the core of the paper contains results for 25\% only.

%\begin{screenonly}
% \subsection{Extended transductive and inductive results on additional Labelled sample proportion}

\begin{figure*}
    \centering
    \subfloat[MPL]{
        \includegraphics[width=0.32\linewidth]{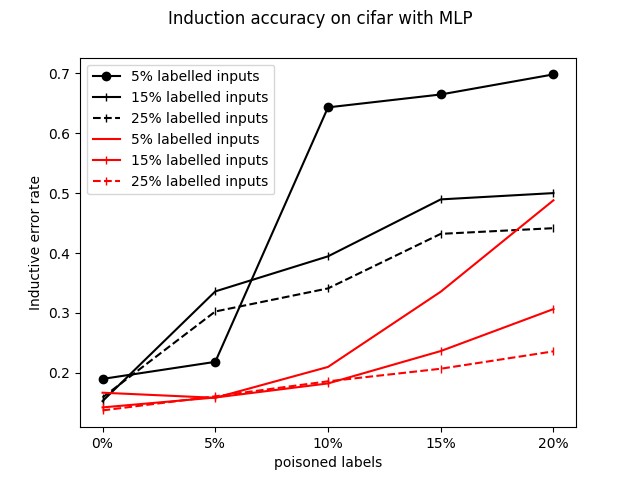} 
        \includegraphics[width=0.32\linewidth]{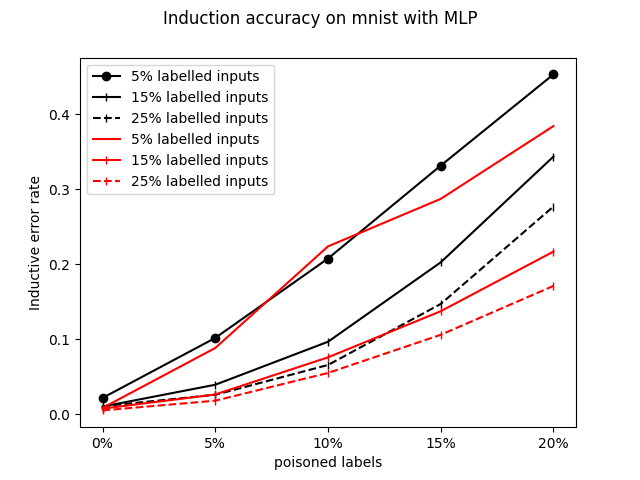}
        \includegraphics[width=0.32\linewidth]{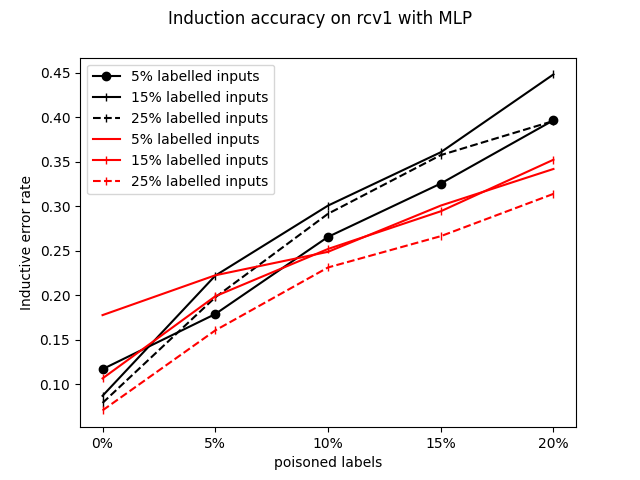}
        } \\
    \subfloat[RFC]{
        \includegraphics[width=0.32\linewidth]{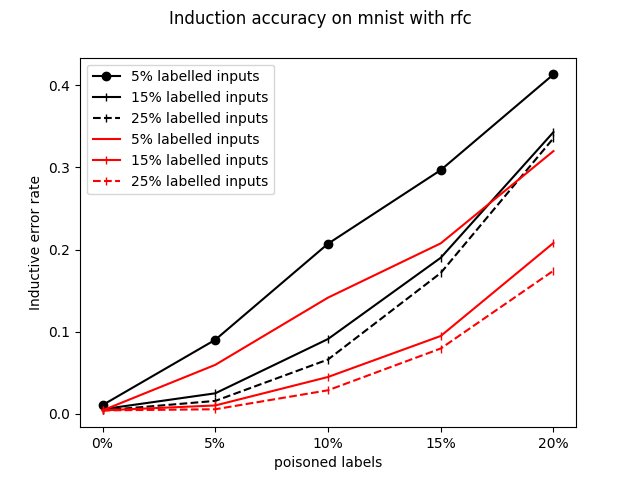} 
        \includegraphics[width=0.32\linewidth]{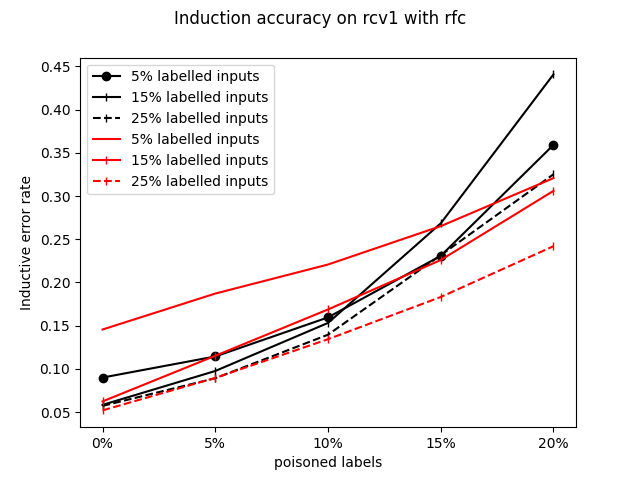}
        \includegraphics[width=0.32\linewidth]{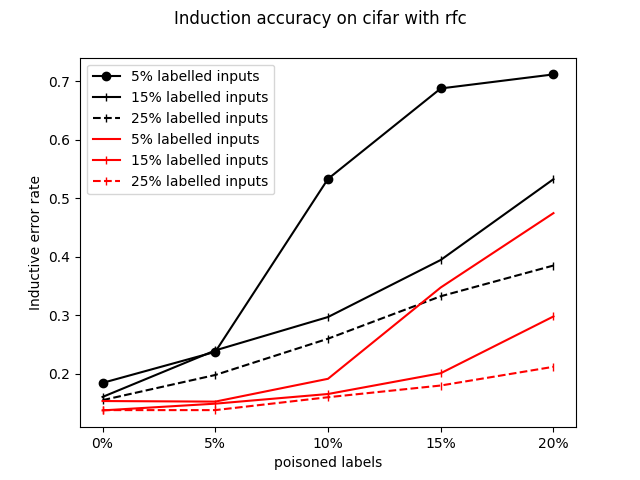}
        }
    % \subfloat[CIFAR]{\includegraphics[width=0.45\linewidth]{figures/rq2_cifar_RF.png} 
    % \includegraphics[width=0.45\linewidth]{figures/rq2_cifar_mlp.png}} \\
    % \subfloat[RCV1]{\includegraphics[width=0.45\linewidth]{figures/rq2_rcv1_RF.png} 
    % \includegraphics[width=0.45\linewidth]{figures/rq2_rcv1_mlp.png}} \\
    \caption{RQ2: Error rate (Y axis) achieved by our data poisoning attack wrt. an increasing poison budget (X axis, expressed in \% of the labelled inputs), measured on random forest classifier (RF, lower row) and multilayer perceptron (MLP, upper row) trained on both known labels and labels inferred with label propagation (black curves) or label spreading (red curves).}
    % \label{fig:rq2}
\end{figure*}

\begin{table*}
    \centering
    \begin{tabular}{|c||c|ccc|ccc|ccc|ccc|}
    \hline
         & no poison & \multicolumn{3}{c|}{5\% labels poisoned} & \multicolumn{3}{c|}{10\% labels poisoned} & \multicolumn{3}{c|}{15\% labels poisoned}
         & \multicolumn{3}{c|}{20\% labels poisoned}\\
         %\hline
         \textbf{MNIST}  & & I & D & S  & I & D & S & I & D & S  & I & D & S \\
         %\hline
         \hline
         5\% labelled & 1.25\% & \textbf{16.22\%} &3.04\%& 5.41\% & \textbf{27.05\%} &3.04\%&9.69\%  & \textbf{35.86\%} &3.04\%&15.13\%  & \textbf{43.98\%}&3.04\%&19.46\% \\
         15\% labelled & 0.69\% &\textbf{16.09\%} & 1.27\%&5.67\% & \textbf{27.48\%} &1.27\%&9.84\% &\textbf{37.07\%} &1.27\%&14.71\% &\textbf{45.71\%} &1.27\% & 20.17\%\\ 
         25\% labelled &0.58\% &\textbf{17.47\%} &1.16\%& 5.68\%  &\textbf{29.94\%} &1.16\%&9.86\% &\textbf{40.26\%} &1.16\%&14.82\% &\textbf{48.88\%} &1.16\%&19.26\% \\ 
         \hline
    \end{tabular}\\
    \vspace{0.2cm}
        \begin{tabular}{|c||c|ccc|ccc|ccc|ccc|}
    \hline
         & no poison & \multicolumn{3}{c|}{5\% labels poisoned} & \multicolumn{3}{c|}{10\% labels poisoned} & \multicolumn{3}{c|}{15\% labels poisoned}
         & \multicolumn{3}{c|}{20\% labels poisoned}\\
         %\hline
         \textbf{CIFAR-10} & & I & D & S  & I & D & S & I & D & S & I & D & S  \\
         %\hline
         \hline
         5\% labelled &19.12\% &\textbf{33.62\%} & 26.15\%&21.90\% &\textbf{53.08\%}& 28.90\% &25.20\% &\textbf{61.67\%}  &28.90\%&25.00\%  &\textbf{66.29\%} &28.90\%& 31.90\% \\
         15\% labelled &17.52\%&\textbf{32.03\%} &26.62\%&18.70\% &\textbf{37.98\%} &26.62\%&19.10\% &\textbf{45.00\%} &26.62\%&26.01\% &\textbf{51.66\%} &26.62\%&28.90\%\\ 
         25\% labelled &17.34\%&\textbf{29.21\%} &28.11\%&19.40\% &\textbf{35.67\%} &28.99\%&20.80\% &\textbf{40.21\%} &28.99\% &19.20\% &\textbf{44.20\%} &28.99\%&21.20\% \\ 
         \hline
    \end{tabular}\\
    \vspace{0.2cm}
        \begin{tabular}{|c||c|ccc|ccc|ccc|ccc|}
    \hline
         & no poison & \multicolumn{3}{c|}{5\% labels poisoned} & \multicolumn{3}{c|}{10\% labels poisoned} & \multicolumn{3}{c|}{15\% labels poisoned}
         & \multicolumn{3}{c|}{20\% labels poisoned}\\
         %\hline
         \textbf{RCV1} & & I & D & S  & I & D & S & I & D & S  & I & D & S  \\
         %\hline
         \hline
         5\% labelled &11.66\% &\textbf{22.22\%} &19.53\% &19.66\% &\textbf{29.39\%}& 28.62\% &28.72\% &\textbf{35.17\%} &34.62\% &35.02\% &\textbf{42.37\%} &38.77\%&39.85\%\\
         15\% labelled &8.19\% &\textbf{22.00\%} &18.13\%&18.69\% &\textbf{31.26\%} &27.09\%&28.01\% &\textbf{38.89\%} &34.74\% &35.28\% &\textbf{46.26\%} &39.10\%&39.96\%\\ 
         25\% labelled &6.91\% &\textbf{23.12\%} &18.41\% &19.31\% &\textbf{33.18\%} &27.98\% &28.22\% &\textbf{41.32\%} &34.62\%&35.15\% &\textbf{49.74\%} &39.57\% &40.12\%\\ 
         \hline
    \end{tabular}
    \caption{RQ3: Error rate (in \%) of \emph{transductive learning} (with label propagation) achieved by our MIR method (I) and the state of the art deterministic (D) and stochastic (S) methods. Higher is better. Bold indicates the best method for each experiment.}
    \label{tab:rq3-effectiveness-transductive-full}
\end{table*}

\begin{table*}
    \centering
    \begin{tabular}{|c||c|ccc|ccc|ccc|ccc|}
    \hline
         & no poison & \multicolumn{3}{c|}{5\% labels poisoned} & \multicolumn{3}{c|}{10\% labels poisoned} & \multicolumn{3}{c|}{15\% labels poisoned}
         & \multicolumn{3}{c|}{20\% labels poisoned}\\
         %\hline
         \textbf{MNIST} & & I & D&S   & I & D&S  & I & D&S  & I & D &S  \\
         %\hline
         \hline
         5\% labelled &1.07\% &\textbf{8.93\%} &1.25\%&0.92\% &\textbf{19.94\%} &1.25\%&1.34\%  &\textbf{29.22\%} &1.25\%&2.64\% &\textbf{40.92\%} &1.25\% &4.35\%\\
         15\% labelled &0.56\% &\textbf{2.27\%} &1.56\%&0.55\% &\textbf{10.31\%} &1.56\%&0.55\%  &\textbf{19.61\%}&1.56\%&0.83\% &\textbf{34.17\%} &1.56\%&1.66\% \\ 
         25\% labelled &0.42\% &\textbf{1.62\%} &0.51\%&0.55\% &\textbf{6.85\%} &1.43\%&0.42\% &\textbf{18.50\%} &1.43\%&0.60\% &\textbf{33.71\%} &1.43\%&1.57\% \\ 
         \hline
    \end{tabular}\\
    \vspace{0.2cm}
        \begin{tabular}{|c||c|ccc|ccc|ccc|ccc|}
    \hline
         & no poison & \multicolumn{3}{c|}{5\% labels poisoned} & \multicolumn{3}{c|}{10\% labels poisoned} & \multicolumn{3}{c|}{15\% labels poisoned}
         & \multicolumn{3}{c|}{20\% labels poisoned}\\
         %\hline
         \textbf{CIFAR-10} & & I & D&S   & I & D&S  & I & D&S  & I & D &S  \\
         %\hline
         \hline
         5\% labelled &18.96\% &22.36\% &\textbf{25.35}\%&17.60\% &\textbf{53.32\%} &28.81\%&19.40\% &\textbf{68.81\%} &28.81\%&20.15\% &\textbf{71.76\%} &28.81\%&21.55\% \\
         15\% labelled &17.25\% &22.10\% &\textbf{24.06}\%&18.55\% &\textbf{29.1\%} &24.04\%&19.25\% &\textbf{43.32\%} & 24.04\%&20.65\% &\textbf{53.45\%} &24.04\%&23.75\% \\ 
         25\% labelled &15.50\% &\textbf{20.55\%} &18.95\%&15.10\% &\textbf{25.70\%} &20.19\%&15.80\% &\textbf{29.60\%} &20.19\%&17.85\% &\textbf{39.90\%} &20.19\%&20.05\% \\ 
         \hline
    \end{tabular}\\
    \vspace{0.2cm}
        \begin{tabular}{|c||c|ccc|ccc|ccc|ccc|}
    \hline
         & no poison & \multicolumn{3}{c|}{5\% labels poisoned} & \multicolumn{3}{c|}{10\% labels poisoned} & \multicolumn{3}{c|}{15\% labels poisoned}
         & \multicolumn{3}{c|}{20\% labels poisoned}\\
         %\hline
         \textbf{RCV1} & & I & D&S   & I & D&S  & I & D&S  & I & D &S  \\
         %\hline
         \hline
         5\% labelled &9.00\% &11.44\% &10.49\%&\textbf{13.79\%}  &15.96\% &16.45\%&\textbf{36.56}\% &23.09\% &26.36\%&\textbf{48.64\%} &35.92\% &29.36\%&\textbf{52.00\%} \\
         15\% labelled &5.85\% &9.77\% &10.85\%&\textbf{13.28\%} &15.33\% &14.22\%&\textbf{38.88\%} &26.84\% &23.38\%&\textbf{51.16\%} &44.08\% &23.38\%&\textbf{53.40\%} \\ 
         25\% labelled &5.73\% & 8.92\% &11.64\%&\textbf{11.68\%} & 13.96\% &20.88\%&\textbf{33.60\%}& 23.17\% &30.08\%&\textbf{50.40\%}&32.60\%& 30.08\%&\textbf{53.40\%} \\ 
         \hline
    \end{tabular}
    \caption{RQ3: Error rate (in \%) of \emph{inductive learning} (with random forest) achieved by our MIR method (I) and the state of the art deterministic (D) and stochastic (S) methods. Higher is better. Bold indicates the best method for each experiment.}
    \label{tab:rq3-effectiveness-inductive-full}
\end{table*}

\begin{table*}
    \centering
    \begin{tabular}{|c||c|ccc|ccc|ccc|ccc|}
    \hline
         & no poison & \multicolumn{3}{c|}{5\% labels poisoned} & \multicolumn{3}{c|}{10\% labels poisoned} & \multicolumn{3}{c|}{15\% labels poisoned}
         & \multicolumn{3}{c|}{20\% labels poisoned}\\
         %\hline
         \textbf{MNIST} & & I & D&S   & I & D&S  & I & D&S  & I & D &S  \\
         %\hline
         \hline
5\% labelled & 2.17\%&\textbf{10.17}\%&3.42\%&2.31\%&\textbf{20.76}\%&3.42\%&2.40\%&\textbf{33.15}\%&3.42\%&5.41\%&\textbf{45.31}\%&3.42\%&7.12\% \\
15\% labelled &0.88\%&\textbf{4.53}\%&1.06\%&1.20\%&\textbf{16.18}\%&1.06\%&1.02\%&\textbf{25.98}\%&1.06\%&1.39\%&\textbf{42.07}\%&1.06\%&2.22\% \\
25\% labelled &0.92\%&\textbf{4.58}\%&1.06\%&0.69\%&\textbf{7.17}\%&1.06\%&0.92\%&\textbf{14.33}\%&1.06\%&1.06\%&\textbf{22.47}\%&1.06\%&1.99\% \\
         \hline
    \end{tabular}\\
    \vspace{0.2cm}
        \begin{tabular}{|c||c|ccc|ccc|ccc|ccc|}
    \hline
         & no poison & \multicolumn{3}{c|}{5\% labels poisoned} & \multicolumn{3}{c|}{10\% labels poisoned} & \multicolumn{3}{c|}{15\% labels poisoned}
         & \multicolumn{3}{c|}{20\% labels poisoned}\\
         %\hline
         \textbf{CIFAR-10} & & I & D&S   & I & D&S  & I & D&S  & I & D &S  \\
         %\hline
         \hline
         5\% labelled &19.00\%&\textbf{21.85}\%&21.80\%&18.80\%&\textbf{64.30}\%&20.15\%&29.70\%&\textbf{66.45}\%&20.15\%&26.90\%&\textbf{69.80}\%&20.15\%&23.90\%\\
15\% labelled &16.85\%&19.05\%&\textbf{31.20}\%&18.10\%&24.25\%&\textbf{32.15}\%&18.60\%&\textbf{44.15}\%&32.15\%&18.05\%&\textbf{51.30}\%&32.15\%&20.25\%\\
25\% labelled &16.50\%&\textbf{17.60}\%&15.95\%&16.90\%&\textbf{19.65}\%&16.85\%&17.45\%&\textbf{27.70}\%&16.85\%&17.30\%&\textbf{40.50}\%&16.85\%&19.65\%\\
         \hline
    \end{tabular}\\
    \vspace{0.2cm}
        \begin{tabular}{|c||c|ccc|ccc|ccc|ccc|}
    \hline
         & no poison & \multicolumn{3}{c|}{5\% labels poisoned} & \multicolumn{3}{c|}{10\% labels poisoned} & \multicolumn{3}{c|}{15\% labels poisoned}
         & \multicolumn{3}{c|}{20\% labels poisoned}\\
         %\hline
         \textbf{RCV1} & & I & D&S   & I & D&S  & I & D&S  & I & D &S  \\
         %\hline
         \hline
5\% labelled&11,68\%&17,88\%&21,16\%&21,52\%&26,56\%&32,00\%&31,72\%&32,56\%&41,08\%&40,68\%&39,68\%&46,24\%&46,92\%\\
15\% labelled&7,40\%&19,16\%&18,92\%&19,00\%&29,08\%&32,92\%&30,04\%&35,88\%&40,76\%&41,28\%&40,48\%&45,04\%&46,56\%\\
25\% labelled&6,72\%&21,12\%&18,96\%&20,28\%&29,48\%&27,64\%&27,44\%&35,32\%&33,68\%&36,56\%&40,80\%&40,08\%&42,64\%\\
         \hline
    \end{tabular}
    \caption{RQ3: Error rate (in \%) of \emph{inductive learning} (with mlp) achieved by our MIR method (I) and the state of the art deterministic (D) and stochastic (S) methods. Higher is better. Bold indicates the best method for each experiment.}
    \label{tab:rq3-effectiveness-inductive-ml-full}
\end{table*}

% \subsection{Extended defence results on additional Labelled samples}
\begin{table*}
    \centering
    \begin{tabular}{|c||ccc|ccc|}
    \hline
         & \multicolumn{3}{c|}{Transduction} & \multicolumn{3}{c|}{Induction}\\
         \textbf{MNIST} & MIR & LAB & None & MIR & LAB & None\\
         \hline
         5\% labelled & \textbf{15.80} & 24.06 & 27.05 & \textbf{04.38} & 12.32 & 19.94 \\
         15\% labelled & \textbf{16.38} & 25.64 & 27.48 & \textbf{01.56} & 06.02 & 10.31 \\
         25\% labelled & \textbf{17.12} & 27.21 & 29.94 &\textbf{01.00} & 03.80 & 6.85 \\
         \hline
    \end{tabular}\\
    \vspace{0.2cm}   
    \begin{tabular}{|c||ccc|ccc|}
    \hline
         & \multicolumn{3}{c|}{Transduction} & \multicolumn{3}{c|}{Induction}\\
         \textbf{CIFAR-10} & MIR & LAB & None & MIR & LAB & None\\
         \hline
         5\% labelled & \textbf{28.76} & 46.06 & 53.08 & \textbf{19.46} & 42.39 & 54.95\\
         15\% labelled & \textbf{23.17} & 36.35 & 37.98 & \textbf{19.47} & 43.44 & 54.11\\
         25\% labelled & \textbf{23.75} & 34.78 & 35.67 & \textbf{17.18} & 41.36 & 44.06\\
         \hline
    \end{tabular}\\
    \vspace{0.2cm}
    \begin{tabular}{|c||ccc|ccc|}
    \hline
         & \multicolumn{3}{c|}{Transduction} & \multicolumn{3}{c|}{Induction}\\
         \textbf{RCV1} & MIR & LAB & None & MIR & LAB & None\\
         \hline
         5\% labelled & \textbf{21.64} & 28.00 & 29.39 & \textbf{10.56} & 13.92 & 15.96\\
         15\% labelled & \textbf{19.58} & 29.62 & 31.26 & \textbf{09.04} & 14.04 & 15.33\\
         25\% labelled & \textbf{20.31} & 31.07 & 33.18 & \textbf{08.20} & 12.24 & 13.96\\
         \hline
    \end{tabular}\\
    \caption{RQ4: Error rate (in \%) achieved by double checking one third of the poisoned labels (MIR) compared with labelling the same number of additional inputs (LAB). Lower is better. None refers to the error rate without countermeasure.}
    \label{tab:rq4-full}
\end{table*}
%\end{screenonly}
